# Supplementary material for: Temperature dependent charge transfer state absorption and emission reveal dominant role of dynamic disorder in organic solar cells
Source: arXiv:2102.06071 source file (2021-05-04)
Supplement: Supplementary file 1 [file goehler2021temperature_SupplementalMaterial.pdf]

# Supplemental material for "Temperature dependent charge transfer state absorption and emission reveal dominant role of dynamic disorder in organic solar cells"

Clemens Göhler, Maria Saladina, Yazhong Wang, Donato Spoltore,
Johannes Benduhn, Karl Leo, and Carsten Deibel

## 1 Device fabrication and materials

The investigated organic solar cells (OSCs) are fabricated with following material layer sequences and thicknesses. Chemical structures and suppliers for the materials are summarized in table S1.

- ITO (90 nm)/ MoO3 (2 nm)/TCTA:$C_{60}$[wt% 10:90] (50 nm)/ BPhen (8 nm)/Al (100 nm)
- ITO (90 nm)/ MoO3 (2 nm)/TAPC:$C_{60}$[wt% 10:90] (50 nm)/ BPhen (8 nm)/Al (100 nm)
- ITO (90 nm)/ MoO3 (2 nm)/TAPC:$C_{60}$[wt% 5:95] (50 nm)/ BPhen (8 nm)/Al (100 nm)

## 2 Power dissipation during electro-optical spectroscopy

With the monochromatic external quantum efficiency ($\mathrm{EQE_{PV}}$) spectroscopy technique, the irradiance on the device under test depends largely on the characteristics of the monochromatic light source, but is usually only a fraction of the solar irradiance. We approximate the absorbed incident power of photons with energy $E_\gamma$ from the measured photocurrent $J(E_\gamma)$ under short circuit conditions. In our experimental setup, without additional bias illumination, maximum photocurrents of $J < 1\,\mu\mathrm{Acm^{-2}}$ are measured under green light. As $\mathrm{EQE_{PV}}$ is measured relative to incident, and not absorbed photons, we find the irradiance for an exemplary $\mathrm{EQE_{PV}}(E_\gamma = 2.4\,\mathrm{eV}) \approx 50\%$:

$$P_{\max} = \frac{J(E_\gamma)}{q \times \mathrm{EQE_{PV}}(E_\gamma)} E_\gamma \approx \frac{1.0\,\mu\mathrm{Acm^{-2}}}{q \times 0.5} \times 2.4\,\mathrm{eV} = 4.8\,\mu\mathrm{Wcm^{-2}} \tag{S1}$$

Thus, during unbiased $\mathrm{EQE_{PV}}$ spectroscopy, we can safely assume to be well below 1 sun solar irradiance of $P_{1\,\mathrm{sun}} = 100\,\mathrm{mWcm^{-2}}$.

Because the emission quantum yield of OSCs is usually very small (record values of less than $4 \times 10^{-3}$[1, 5] were reported OSCs with non-fullerene acceptors), the solar cell is driven at high forward bias during electroluminescence (EL) spectroscopy to inject comparably large driving currents. In our case, we applied injection currents in the range of $J_{\mathrm{inj}}(V_{\mathrm{bias}} \approx 1\,\mathrm{V}) \approx 150\,\mathrm{mAcm^{-2}}$. The total dissipated electrical power of

Table S1: Materials used in the active layer blend and device stack with chemical structures and supplier.

| Function | Abbr. | Chemical structure | Supplier |
|---|---|---|---|
| electron donor | TCTA | 4,4',4"-Tris(carbazol-9-yl)triphenylamine 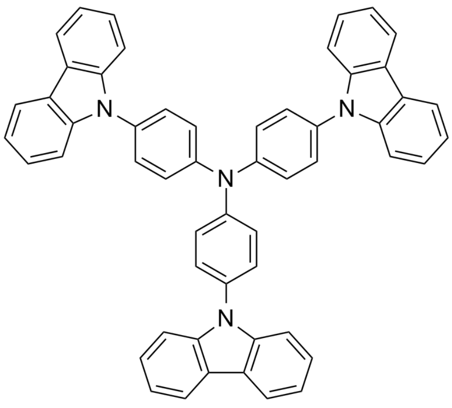 | Sensient Technologies Corporation, USA |
| electron donor | TAPC | 1,1-bis[4-(N,N-di-ptolylamino)phenyl]cyclohexane 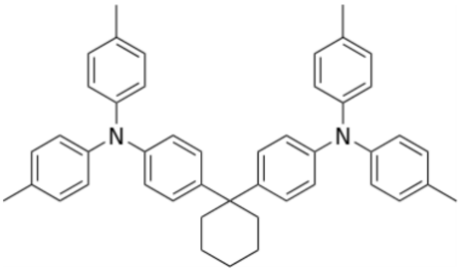 | Sensient Technologies Corporation, USA |
| electron acceptor | $C_{60}$ | ($C_{60}$-$I_h$)[5,6]fullerene 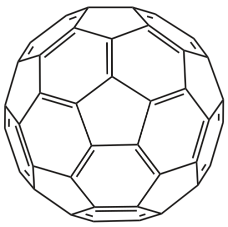 | CreaPhys GmbH, Germany<br>or<br>Luminescence Technology Corp. (Lumtec), Taiwan |
| hole transport layer | $MoO_3$ | Molybdenum trioxide | Luminescence Technology Corp. (Lumtec), Taiwan |
| electron transport layer | BPhen | Bathophenanthroline (4,7-diphenyl-1,10-phenanthroline) 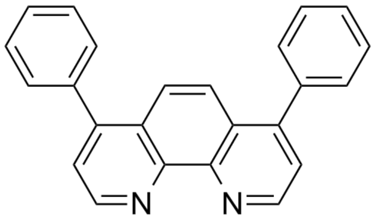 | Abcr GmbH, Germany<br>or<br>Luminescence Technology Corp. (Lumtec), Taiwan |

$P_{EL} \approx 150\,\mathrm{mWcm^{-2}}$ exceeds the incident irradiance from solar irradiation, and since emission yields are very low for OSCs, most of the dissipated power will be thermalized. Even more so, as not every incident photon from the sun would be absorbed by the solar cell, but most absorbed photons yield charge carriers due to good internal quantum efficiencies even in the low-absorbing spectral range.[4, 2] Based on these considerations, we would expect unintended heating of the solar cells to occur most likely during EL spectroscopy.

# 3 Heating of devices during EL–measurements

When we look at $EQE_{EL}$–spectra from solar cells with varying donor content, we find unexpected, significant differences of the distribution width at lower temperatures. Fig. S1 shows these findings for TAPC:$C_{60}$ solar cells with 5% and 10% donor content. The spectral shape of the 5%–cell seems much less affected by temperature. This effect is usually attributed to a larger amount of static energetic disorder. The emission line width would remain more static in this case; we would also expect a temperature dependent peak shift which is missing here.

However, before we can trust these conclusions, we need to make sure that the emission temperature is indeed equal to the set temperature of the apparatus. As shown in the study, the analysis of electro-optical reciprocal $EQE_{PV}$– and $EQE_{EL}$–spectra suggest otherwise: the emission temperature of the 5%–device may be increased during $EQE_{EL}$–measurements.

The low EL–emission quantum yield of organic solar cells usually requires high injection current densities to gain a reasonable signal for emission spectroscopy. High current densities are an additional source of heating, which may lead to a higher emission temperature of the device. With the electro–optical reciprocity relation and a $EQE_{PV}$–spectra at $T_{set}$, were are able to compare the emission temperature $T_{valid}$ to $T_{set}$. If both temperatures are not equal, we imply reasonable doubt of the emission temperature. In Fig. S2, we show that the difference of $T_{valid}$ and $T_{set}$ correlates with the injection current density of a device; the difference increases at lower temperatures $T_{set}$, while almost vanishing at room temperature. These findings highlight the necessity of some form of control mechanism for emission temperatures, especially when operating at low device temperatures.

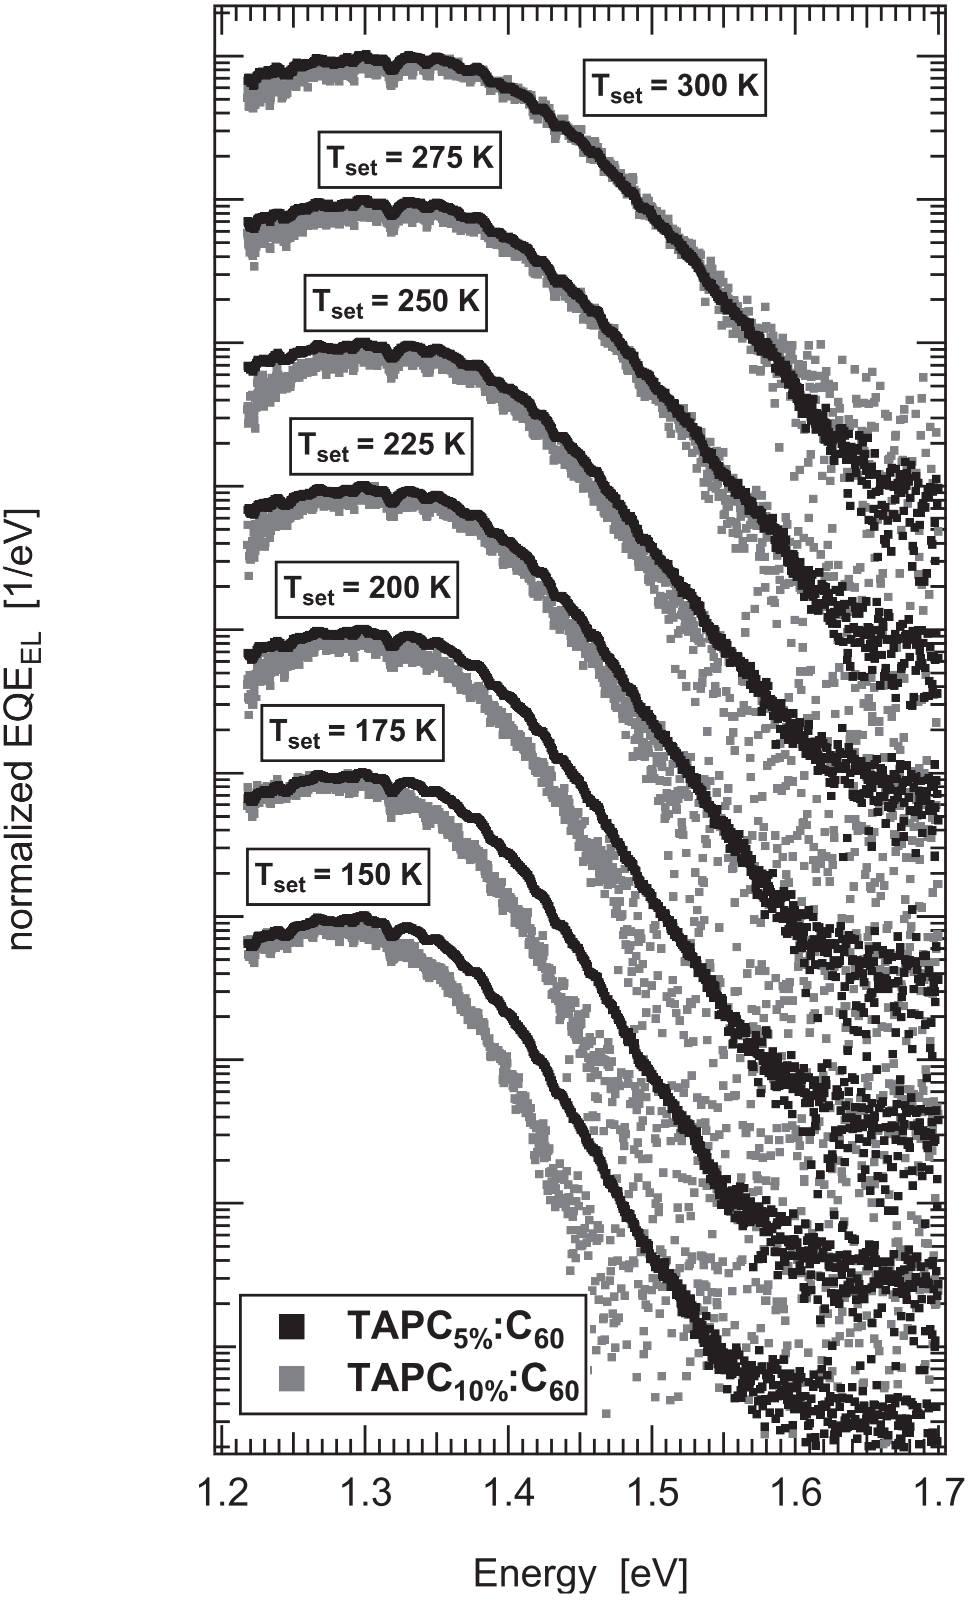


Figure S1: $EQE_{EL}$ spectra from TAPC:$C_{60}$ solar cells with 5% and 10% donor content. While the emission spectra overlap at $T_{set} > 250\,K$, we see a faster linewidth-reduction for the 10% cell compared to the other. This indicates to a higher device temperature of the 5% cell in the low temperature range; other interpretations could be a significant higher amount of static energetic disorder in the low-content cell (which would lead to a more static emission linewidth, albeit the emission peak shift is missing).

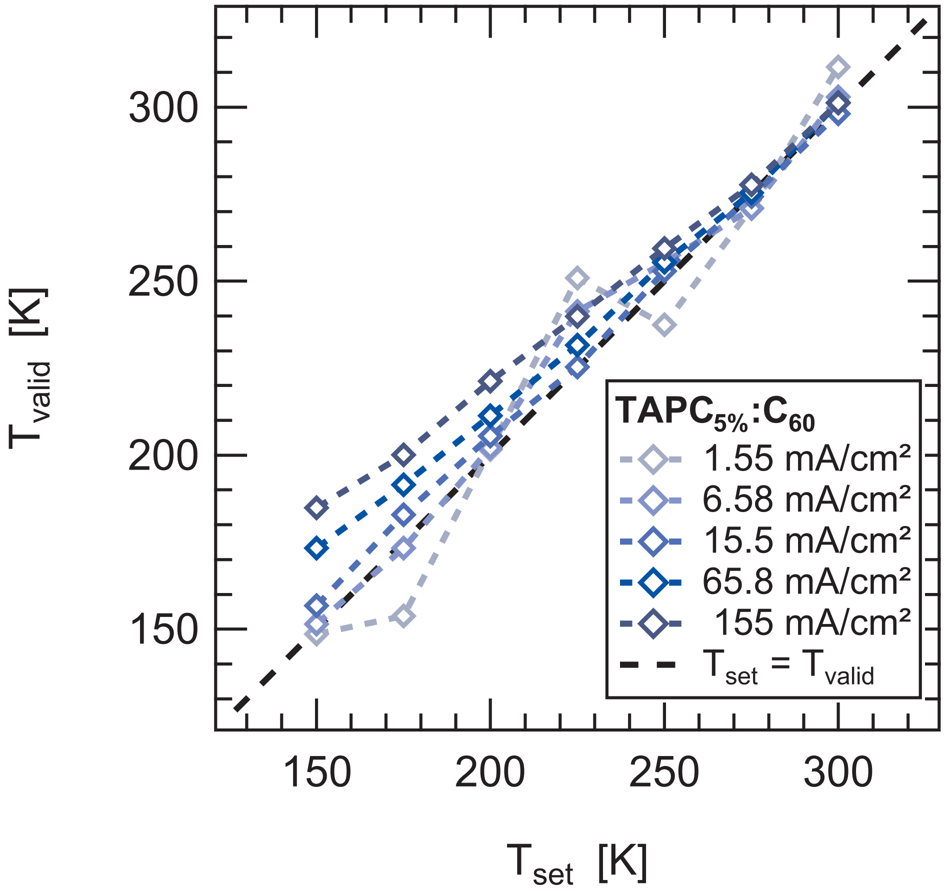


Figure S2: Effect of the injection current density $J_{\text{inj}}$ on the validated reciprocity temperature $T_{\text{valid}}$ for TAPC:$C_{60}$ solar cell with 5% donor content. The analysis is based on a set of $\text{EQE}_{\text{EL}}$–spectra: with the sample being held at $T_{\text{set}}$, emission spectra with exponentially increasing $J_{\text{inj}}$ were recorded with constant integration time. Increasing the injection current correlates with an increased $T_{\text{valid}}$. The effect becomes more pronounced at lower $T_{\text{set}}$. All spectra were analyzed as reciprocal to one $\text{EQE}_{\text{PV}}$–spectrum recorded at the same $T_{\text{set}}$. Emission spectra at smaller injection currents show a lower signal–to–noise ratio, which results in individual outliers at $J_{\text{inj}} = 1.55\,\text{mAcm}^{-2}$.

## 4 Differences between *multiple vibrations model* and *extended disordered Marcus model*

In Fig. S3 we show calculated $\mathrm{EQE_{PV}}$ and $\mathrm{EQE_{EL}}$ spectra between $T = 50...300\,\mathrm{K}$ to illustrate fundamental differences between the influence of broadening by static and dynamic energetic disorder on characteristic spectral properties. We used comparable parameters for both models, which are listed Table S2, and omitted any donor or acceptor singlet states.

| | edM | mV |
|---|---|---|
| $E_{\mathrm{ct}}$ | 1.40 eV | |
| $\lambda_{\mathrm{R}}$ | 70 meV | |
| $S$ | 2.5 | |
| $\Lambda_{\mathrm{vibr}}$ | 150 meV | |
| $\sigma_{\mathrm{ct}}$ | 40 meV | - |
| $S_2$ | - | 5.0 |
| $\Lambda_2$ | - | 13.0 meV |

Table S2: Model parameters used to calculate temperature dependent CT $\mathrm{EQE_{PV}}$ and $\mathrm{EQE_{EL}}$ spectra in Fig. S3 according to the *extended disordered Marcus model* (edM) and *multiple vibrations model* (mV).

We can see right away that the statically disordered $\mathrm{EQE_{EL}}$ spectra feature a strong temperature induced peak shift towards lower energies. Static energetic disorder also reduces the formation of a distinct high–energetic vibration substructure in $\mathrm{EQE_{PV}}$ spectra. While not as pronounced, a similar $\mathrm{EQE_{EL}}$ shift occurs in the *multiple vibrations model*; the peak positions of both models are shown in Fig. S4.

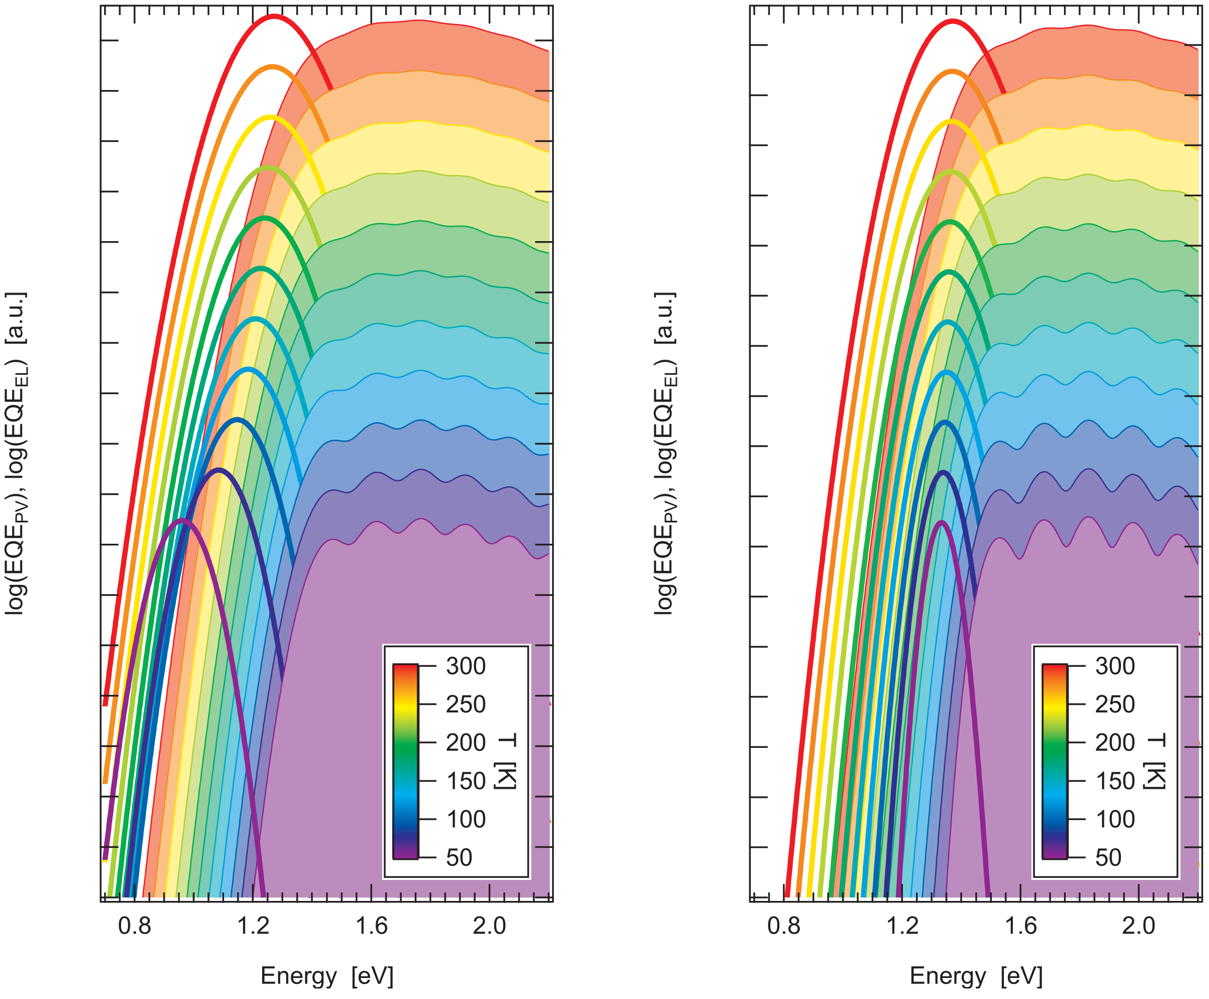


(a) extended disordered Marcus model

(b) multiple vibrations model

Figure S3: Calculated temperature dependent CT state contribution to $EQE_{PV}$ (filled curves) and $EQE_{EL}$ (solid lines) spectra according to the (a) *extended disordered model* and (b) *multiple vibrations model*.

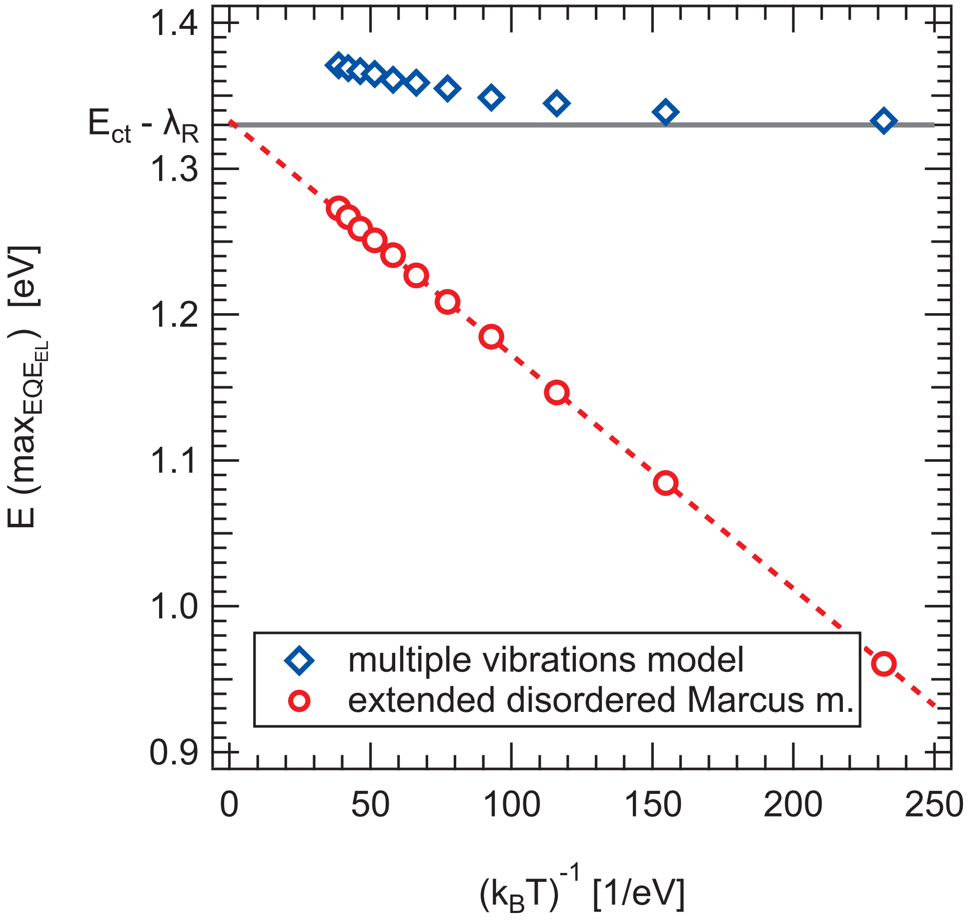


Figure S4: Calculated maximum position $E(\max_{\mathrm{EQE_{EL}}})$ of the temperature dependent $\mathrm{EQE_{EL}}$ peak for the *extended disordered model* and the *multiple vibrations model*. In the statically disordered model, we find the peak shift proportional to $1/k_{\mathrm{B}}T$ (dashed line), with the slope defined by the distribution variance $\sigma_{\mathrm{ct}}^2$. The emission peak shift due to dynamic broadening in the *multiple vibrations model* is comparably smaller and not linear with $1/k_{\mathrm{B}}T$. The peak shifts depend on the used model parameters, yet we find a fundamental difference in their respective limit: in the *extended disordered model*, the peak maximum reaches $E_{\mathrm{ct}} - \lambda_{\mathrm{R}}$ (the theoretical value from the *simple Marcus model*) at high temperatures as illustrated by the extrapolated dashed line, while the same value is the low-temperature limit in the *multiple vibrations model*.

# 5 Individual peak analysis

CT distributions in the reduced $EQE_{PV}$ and $EQE_{EL}$ spectra were fitted individually with a Gaussian lineshape according to the *disordered Marcus model* (Equations (8) and (9)). We opted for a numerical reconstruction of the spectral data with Equations (S2) and (S3) to avoid non-linear fitting and instead implement a linear regression.[3] The energy independent terms $B_{EQE}(T)$ and $B_{EL}(T)$ can be used to calculate $E_{ct}$.

$$\frac{\delta}{\delta E}\ln\left(E \times \mathrm{EQE_{PV}}\right) \propto \frac{E_{ct}+\lambda_R}{\sigma_{ct}^2+2\lambda_R k_B T} - \frac{E}{\sigma_{ct}^2+2\lambda_R k_B T} = B_{PV} + \frac{E}{\sigma_{PV}^2(T)} \tag{S2}$$

$$\frac{\delta}{\delta E}\ln\left(\frac{\mathrm{EQE_{EL}}}{E}\right) \propto \frac{E_{ct}-\lambda_R-\frac{\sigma_{ct}^2}{k_B T}}{\sigma_{ct}^2+2\lambda_R k_B T} - \frac{E}{\sigma_{ct}^2+2\lambda_R k_B T} = B_{EL} + \frac{E}{\sigma_{EL}^2(T)} \tag{S3}$$

The temperature dependence of the Gaussian linewidth $\sigma^2(T)$ can be used to determine the reorganization energy $\lambda_R$ and the width $\sigma_{ct}$ of the statically disordered $E_{ct}$ distribution; if $\sigma_{ct} = 0$, this method directly translates to the *simple Marcus model.* As we only investigate the slope regions of the spectra, this method is not sensitive for extended models with characteristic vibrations. Tvingstedt et al. have discussed how this analysis would effect the outcomes on an underlying *multiple vibrations model.*[3] Fig. S5 shows individual peak widths $\sigma^2$ for both emission and absorption of $TCTA_{10\%}$:$C_{60}$.

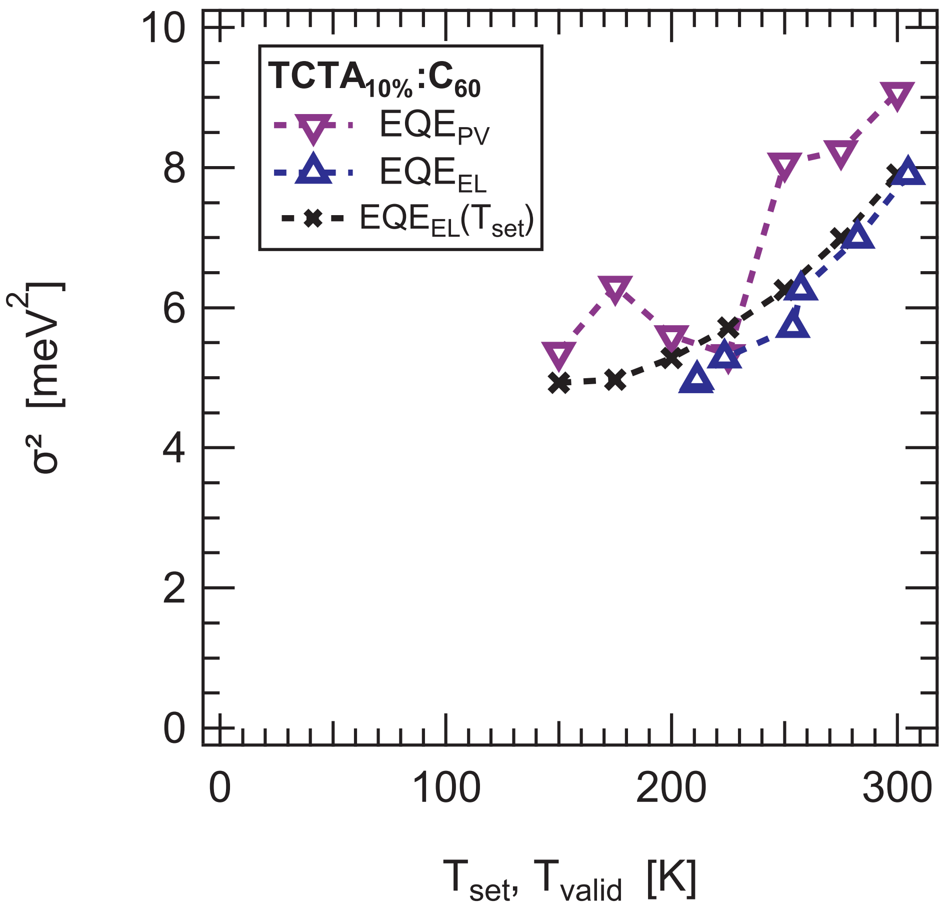


Figure S5: Individual CT line variances $\sigma^2$ for temperature dependent $EQE_{PV}$ and $EQE_{EL}$ spectra of $TCTA_{10\%}$:$C_{60}$, with regard to the expected temperature $T_{set}$ and the device temperature $T_{valid}$ (dashed lines given as guide to the eye). The extracted values from individual analysis of $EQE_{PV}$ lines show more scatter than for TAPC:$C_{60}$ devices, which may be connected to the less pronounced CT absorption lines due to a lower offset between singlet and CT state absorption.

## 6 Extrapolated $V_{oc}$ limitation at $T = 0\,\mathrm{K}$

By measuring the temperature dependent open-circuit voltage at increasing generation rate $G$ and extrapolating the linear trend of $V_{oc}(T, G = \mathrm{const.})$ towards $T = 0\,\mathrm{K}$, we are able to determine the open circuit voltages limit for each solar cell; respective measurement results for all devices are shown in Fig. S7(a-c).

Non-linear trends are observed within two major limitations: the shunt resistance interferes with the voltage measurement especially at low temperatures and low incident LASER intensities, and a high LASER power causes additional heating of the devices. The high number of data points for each device allows us to calculate local derivatives of the curves instead of performing long-range linear fits. Afterwards, we determine the $V_{oc}$ limit as the 1st moment of a normal distribution over all locally extrapolated values (see Fig. S7d).

One might argue that the measured data points from non-linear curves could affect the resulting distribution of locally derived $V_{oc}$–limits, and should therefore be excluded from analysis. We have addressed this issue by performing the same distribution analysis while reducing the number of involved $V_{oc}$ curves one-by-one, until we are left within a hand-selected range of trusted values. An exemplary analysis for all devices is shown in Fig. S6. Keep in mind that most shunt-limited voltages will yield local $V_{oc}$ limits below $1\,\mathrm{V}$ and would already be excluded from the distribution. We find shifts of the distribution center by $\pm 10...20\,\mathrm{meV}$; however, the selection of the trusted region can strongly affect the outcome. Therefore, we prefer to use unfiltered data to obtain $V_{oc}$–limits, and keep an uncertainty of $\Delta V_{oc}(T \to 0\,\mathrm{K}) = \pm 20\,\mathrm{meV}$ (less than 2% relative uncertainty).

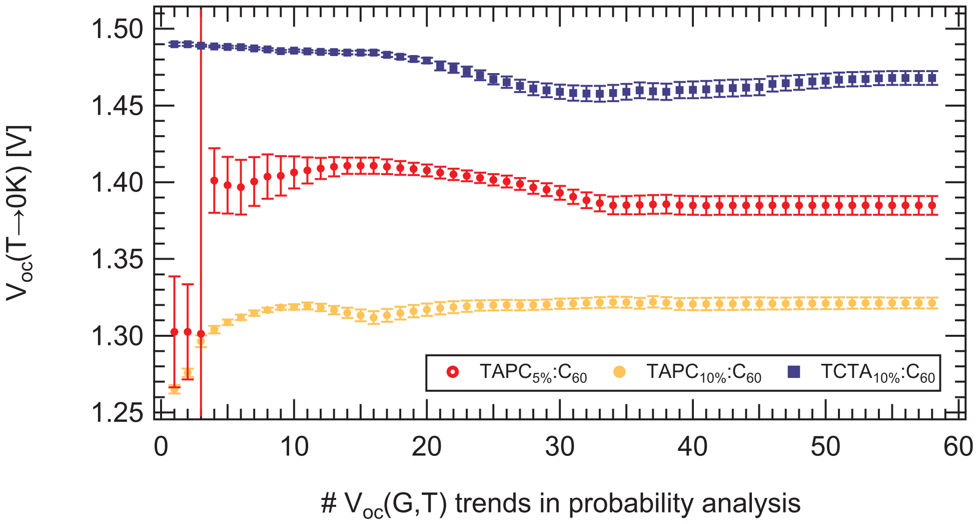


Figure S6: Center of the distribution of extrapolated $V_{oc}(T \to 0\,\mathrm{K})$ values from temperature dependent $V_{oc}(G)$ measurements (shown in Fig. S7), while reducing the number of included measured values. Error bars illustrate respective standard deviations of the distribution. Depending on the selected range of trusted values the manifold of measured voltages, the distribution center might shift by some $10\,\mathrm{meV}$.

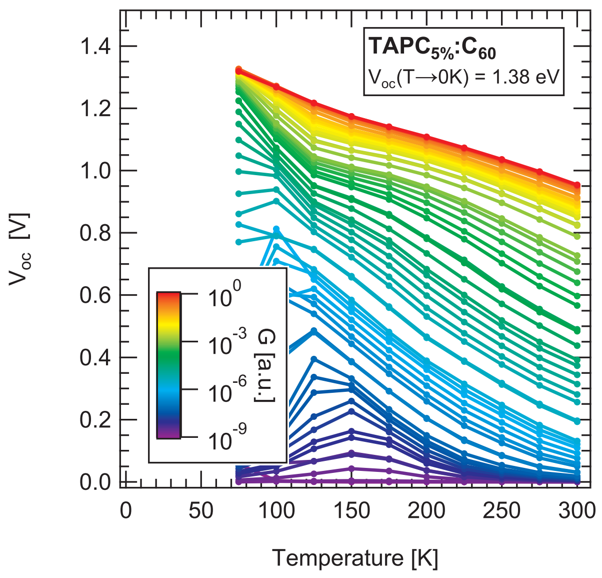


(a)

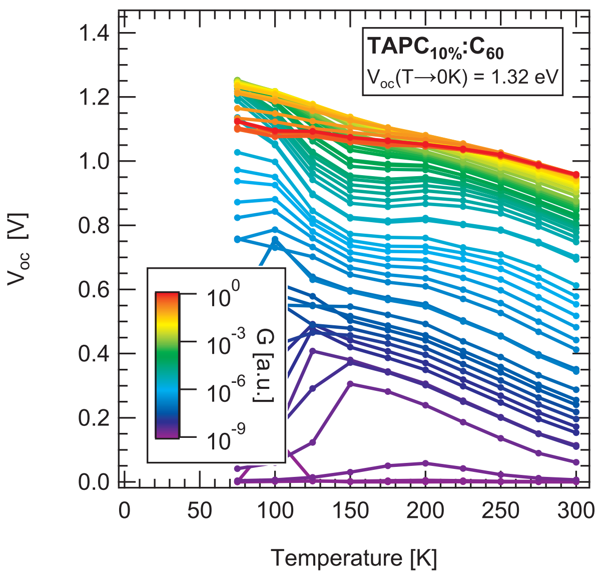


(b)

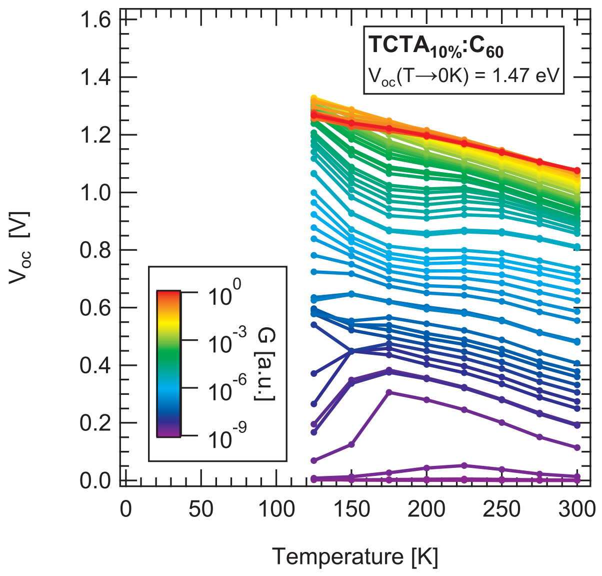


(c)

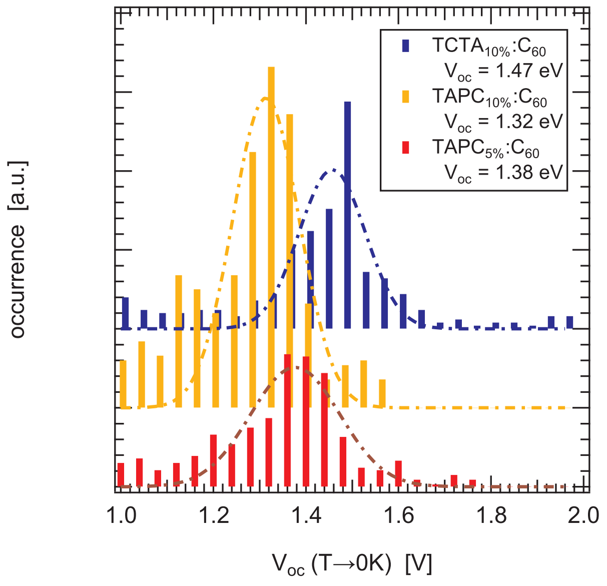


(d)

Figure S7: (a-c) open circuit voltage $V_{oc}$ for increased incident light power (color-coded) and device temperature $T_{set}$. (d) Distribution of locally extrapolated $V_{oc}$-limits at $T = 0\,K$, and first moment of the distribution.

# 7 Non-linear least square fit results

We fitted each of the $\mathrm{EQE_{PV}}$ and $\mathrm{EQE_{EL}}$ spectra collectively with a joint set of parameters; the results of which are shown in Table S3. The temperature of each spectrum was held constant at $T_{\mathrm{set}}$ (for $\mathrm{EQE_{PV}}$ data) and $T_{\mathrm{valid}}$ (for $\mathrm{EQE_{EL}}$ data), respectively. A variable amplitude was allocated to every measurement as the only individual parameter (not shown here).

The fit algorithm is based on the open-source `lmfit`-package (`v1.0.0`) for Python 3.x. It weighted the residuals of each individual spectrum equally. This was necessary to avoid overrating of $\mathrm{EQE_{EL}}$ spectra (which have more supporting data points compared to $\mathrm{EQE_{PV}}$ measurements) and measurements taken at higher temperatures (which have more supporting data points due to a better signal–to–noise ratio and broader linewidths). Therefore, each spectrum's residual is divided by its share $n_i$ in the entire number of supporting points:

$$n_i = \frac{\#\ \text{supporting points in spectrum}\ i}{\#\ \text{supporting points overall}} \tag{S4}$$

**The parameter $\Lambda_{\mathrm{vibr}}$ was held constant at $150\,\mathrm{meV}$ for every model involving the high frequency vibration; the value represents the lower limit of the reported range of carbon-carbon stretch vibration energies. Varying this parameter over the full reported range $150\ldots180\,\mathrm{meV}$ (not shown) did not significantly affect the fit quality or extracted parameters. For every model involving a progression of vibrational modes, the respective sums were calculated up to $20$ terms ($j = 0\ldots19$) for the high energy vibration, and $300$ terms ($i = 0\ldots299$) for the low energy vibration (resulting in $i \cdot j = 6000$ terms for the multiple vibration model).**

Both the extended disordered Marcus (edM) model and multiple vibrations (mv) model can satisfyingly fit the broadened $\mathrm{EQE_{PV}}$-spectra at low temperatures and intermediate region between $E_{\mathrm{ct}}$ and the $C_{60}$bandgap. Only the mv-model is capable to explain $\mathrm{EQE_{EL}}$ spectra, which might be due to one more parameter ($S_2$ and $\Lambda_2$ compared to $\sigma_{\mathrm{ct}}$) included in the model. The asymmetry between $\mathrm{EQE_{PV}}$ and $\mathrm{EQE_{EL}}$ is indeed better described by a Poisson distribution characterized by $S_2$ and $\Lambda_2$, than simple temperature independent broadening provided by the static parameter $\sigma_{\mathrm{ct}}$. However, the other main reason the mv-model results in better fits is its much smaller electroluminescence peak shift limited towards $E_{\mathrm{ct}}$ (illustrated in Fig. S4). In comparison, static energetic disorder implies an increasing EL peak shift towards lower temperatures regardless of $E_{\mathrm{ct}}$, which is not consistent with experimental data.

Table S3: Extracted fit parameters for combined temperature dependent CT state $EQE_{PV}$ and $EQE_{EL}$ characteristics according to the *simple* (sM), *disordered* (dM), *extended* (eM), and *extended disordered Marcus model* (edM), and the *multiple vibrations model* with two characteristic vibrations (mV). The high-frequency vibration $\Lambda_{vibr}$ was held constant at an energy of 150 meV, which corresponds to the characteristic vibration of the fullerene acceptor.

| parameter | $TAPC_{5\%}$ | | | | | $TAPC_{10\%}$ | | | | | $TCTA_{10\%}$ | | | | |
|---|---|---|---|---|---|---|---|---|---|---|---|---|---|---|---|
| | sM | dM | eM | edM | mV | sM | dM | eM | edM | mV | sM | dM | eM | edM | mV |
| $E_{ct}$/eV | 1.40 | 1.47 | 1.39 | 1.47 | 1.33 | 1.42 | 1.52 | 1.40 | 1.48 | 1.38 | 1.47 | 1.66 | 1.45 | 1.60 | 1.34 |
| $\lambda_R$/meV | 135 | 67 | 94 | 68 | 93 | 124 | 71 | 109 | 73 | 114 | 146 | 51 | 121 | 62 | 132 |
| $\sigma_{ct}$/meV | - | 61 | - | 48 | - | - | 48 | - | 46 | - | - | 85 | - | 73 | - |
| $\Lambda_{vibr}$/meV | - | - | | *150* | | - | - | | *150* | | - | - | | *150* | |
| $S$/1 | - | - | 5.3 | 3.3 | 2.2 | - | - | 5.0 | 2.7 | 2.0 | - | - | 10.0 | 6.1 | 3.5 |
| $\Lambda_2$/meV | - | - | - | - | 13.7 | - | - | - | - | 12.5 | - | - | - | - | 7.1 |
| $S_2$/1 | - | - | - | - | 2.3 | - | - | - | - | 8.9 | - | - | - | - | 18.2 |

## 8 Comparison of predicted $EQE_{LED}$

In Fig. S8 we compared relative integrated $EQE_{LED}$ values from the measured spectra with model fits.

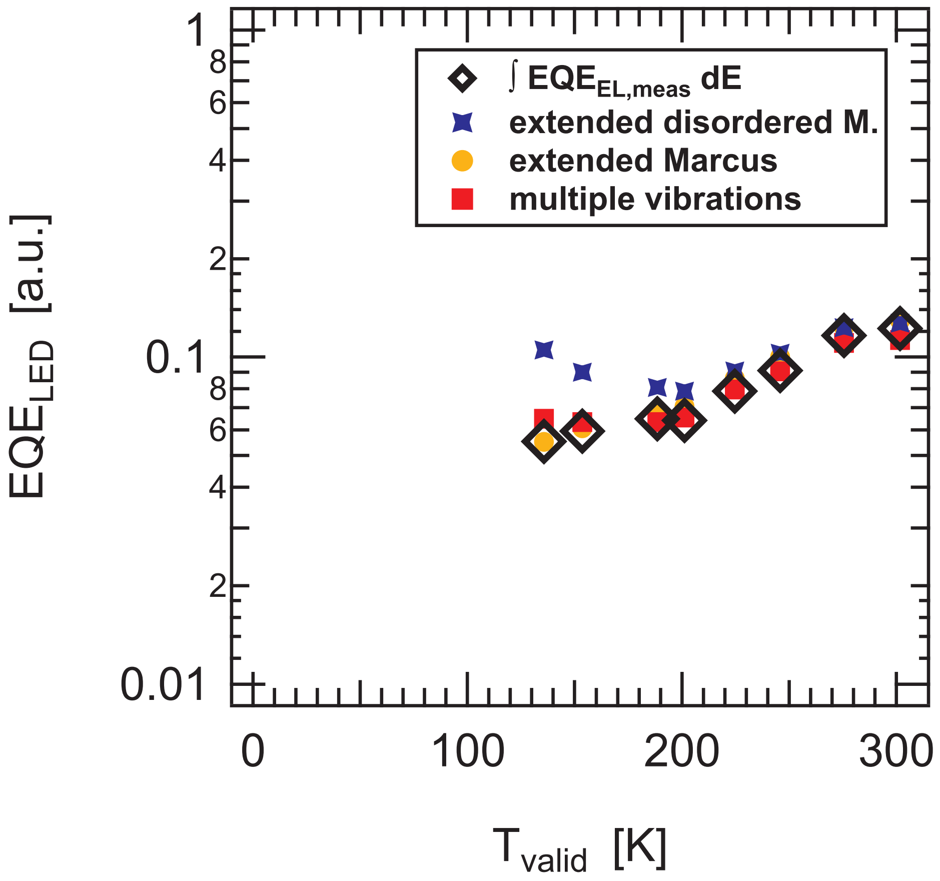


Figure S8: Approximated EL emission quantum yield $EQE_{LED}$ from integrated measured (open diamonds) and fitted $EQE_{EL}$ spectra according to different models. We find an increasing deviation for $T_{valid} <$ 250 K in the predicted $EQE_{LED}$ values of the *extended disordered model*, while models without static disorder do match the measured values.

# 9 Rescaled $EQE_{PV}$ and $EQE_{EL}$ data

In Fig. S9, we have rescaled the measured $EQE_{PV}(E, T)$ and $EQE_{EL}(E, T)$ data from Fig. 1 to match at their normalized maximum, and increased the zoom level to the perceived CT region of the $EQE_{PV}$.

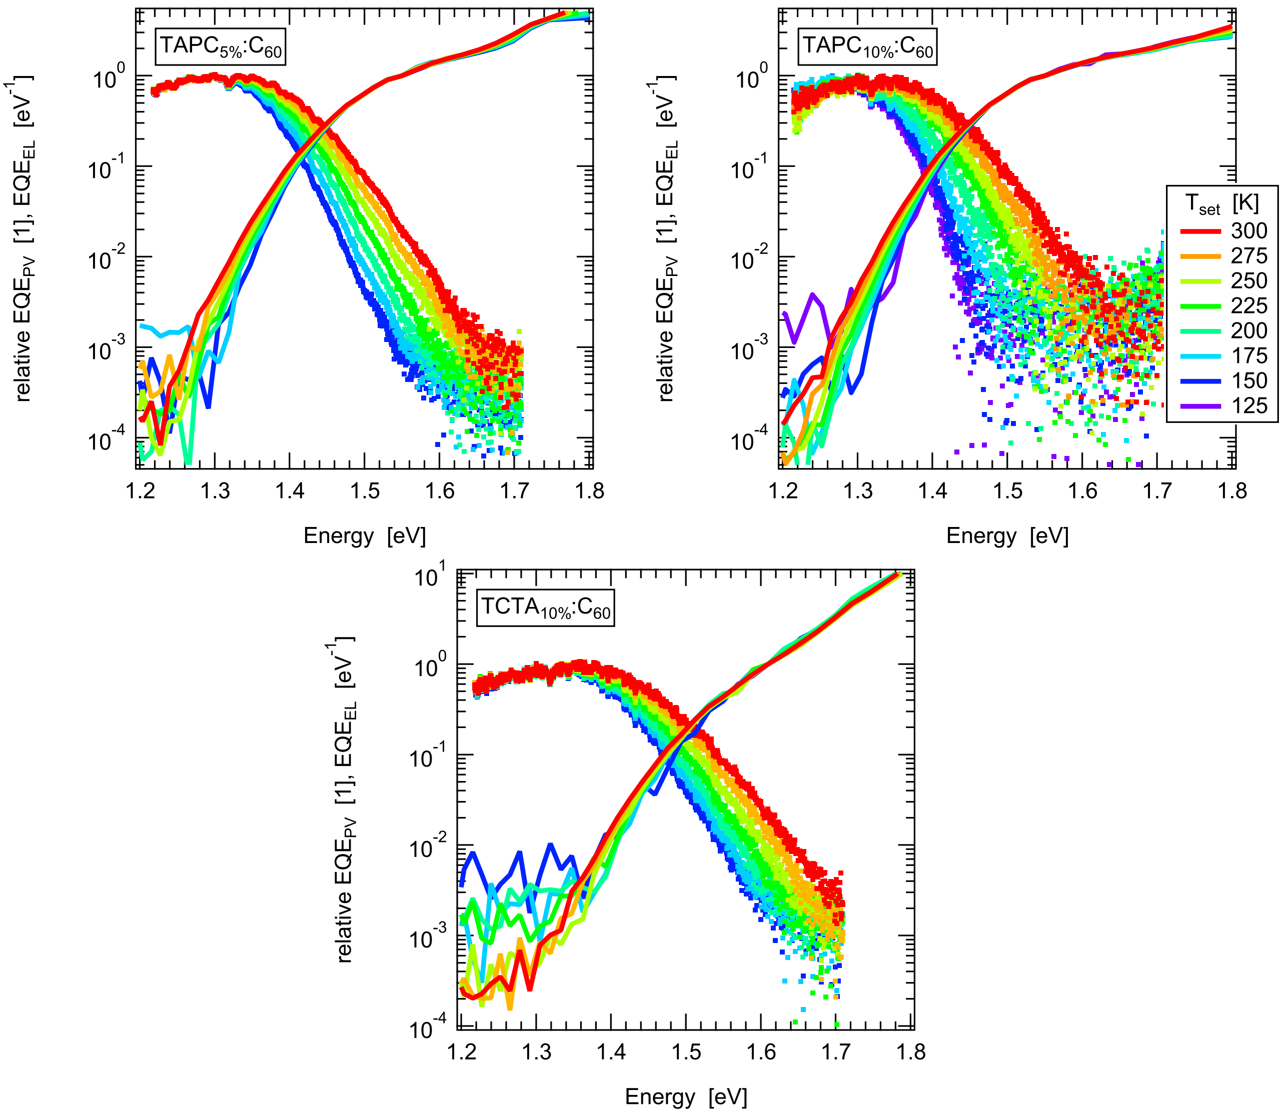


Figure S9: Measured relative $EQE_{PV}$ and $EQE_{EL}$ spectra for (a) TAPC:$C_{60}$ bulk heterojunction solar cells with 5 wt% and (b) 10 wt% donor content, and (c) TCTA:$C_{60}$ bulk heterojunction solar cell with 10 wt% donor content. All measured curves were normalized to their perceived maxmima.

# References


[1] Martin A Green and Anita WY Ho-Baillie. Pushing to the limit: radiative efficiencies of recent mainstream and emerging solar cells. *ACS Energy Letters*, 4(7):1639–1644, 2019.

[2] Maria Saladina, Simon Marques, Anastasia Markina, Safakath Karuthedath, Christopher Wöpke, Clemens Göhler, Yue Chen, Magali Allain, Philippe Blanchard, Clement Cabanetos, Denis Andrienko, Frederic Laquai, Julien Gorenflot, and Carsten Deibel. Charge photogeneration in non-fullerene organic solar cells: Influence of excess energy and electrostatic interactions. *Advanced Functional Materials*, -(-):2007479, 2020.

[3] Kristofer Tvingstedt, Johannes Benduhn, and Koen Vandewal. Temperature dependence of the spectral line-width of charge-transfer state emission in organic solar cells; static vs. dynamic disorder. *Materials Horizons*, 7:1888–1900, 2020.

[4] Koen Vandewal, Steve Albrecht, Eric T Hoke, Kenneth R Graham, Johannes Widmer, Jessica D Douglas, Marcel Schubert, William R Mateker, Jason T Bloking, George F Burkhard, Alan Sellinger, M J Fréchet, Aram Amassian, Moritz K Riede, Michael D McGehee, Dieter Neher, and Alberto Salleo. Efficient charge generation by relaxed charge-transfer states at organic interfaces. *Nature Materials*, 13(1):63–68, 2014.

[5] Yuan Xie, Weiping Wang, Wei Huang, Fengyuan Lin, Tengfei Li, Sha Liu, Xiaowei Zhan, Yongye Liang, Chao Gao, Hongbin Wu, and Yong Cao. Assessing the energy offset at the electron donor/acceptor interface in organic solar cells through radiative efficiency measurements. *Energy & Environmental Science*, 12(12):3556–3566, 2019.
